# Supplementary material for: Is the protactinium(V) mono-oxo bond weaker than what we thought?
Source: arXiv:2409.01338 source file (2024-10-07)
Supplement: Supplementary file 1 [file supp-pao-bond.pdf]

# Supporting Information:

## Is the protactinium(V) mono-oxo bond weaker than what we thought?

Tamara Shaaban,<sup>†</sup> Hanna Oher,<sup>‡</sup> Jean Aupiais,<sup>¶</sup> Julie Champion,<sup>§</sup> André Severo Peirera Gomes,<sup>†</sup> Claire Le Naour,<sup>‡</sup> Melody Maloubier,<sup>‡</sup> Florent Réal,<sup>†</sup> Eric Renault,<sup>||</sup> Xavier Rocquefelte,<sup>⊥</sup> Bruno Siberchicot,<sup>¶</sup> Valérie Vallet,<sup>†</sup> and Rémi Maurice\*,<sup>⊥</sup>

<sup>†</sup>*Univ. Lille, CNRS, UMR 8523 - PhLAM - Physique des Lasers Atomes et Molécules, F-59000 Lille, France*

<sup>‡</sup>*Université Paris-Saclay, CNRS/IN2P3, IJCLab, 91405 Orsay, France*

<sup>¶</sup>*CEA, Laboratoire Matière en Conditions Extrêmes, Université Paris-Saclay, F-91680, Bruyères-le-Châtel, France; CEA, DAM, DIF, 91297 Arpajon, France*

<sup>§</sup>*IMT Atlantique, Nantes Université, CNRS/IN2P3, SUBATECH, F-44000 Nantes, France*

<sup>||</sup>*Nantes Université, CNRS, CEISAM UMR 6230, F-44000 Nantes, France*

<sup>⊥</sup>*Univ Rennes, CNRS, ISCR (Institut des Sciences Chimiques de Rennes) – UMR 6226, F-35000 Rennes, France*

E-mail: remi.maurice@univ-rennes.fr

# List of Tables

|    |                                                                                                                                                                                                                                                                                                                                                       |      |
|----|-------------------------------------------------------------------------------------------------------------------------------------------------------------------------------------------------------------------------------------------------------------------------------------------------------------------------------------------------------|------|
| S1 | Integrated crystal orbital bond indices (ICOBIs) <sup>S1</sup> obtained at the optimized structures (see Tables 1 and 2). Mean values are reported when related bonds are crystallography independent. . . . .                                                                                                                                        | S-4  |
| S2 | Benchmark of ten exchange-correlation (XC) functionals based on the Abinit code <sup>S2</sup> for selected protactinium molecular systems. Only the Pa–O bond distance (Å) is reported. . . . .                                                                                                                                                       | S-5  |
| S3 | Role of implicit solvation (C-PCM <sup>S3</sup> ) on the Pa–O bond distance (Å) obtained with Gaussian <sup>S4</sup> and the default radii (UFF <sup>S5</sup> ). . . . .                                                                                                                                                                              | S-6  |
| S4 | Role of implicit solvation (COSMO <sup>S6</sup> ) on the Pa–O bond distance (Å) obtained with ADF <sup>S7</sup> and the default radii. <sup>S8</sup> The ZORA <sup>S9</sup> Hamiltonian was used. Values in red are reported from the main text for convenience. . . . .                                                                              | S-7  |
| S5 | Role of implicit solvation (COSMO <sup>S6</sup> ) on the U–O bond distance(s) (Å) obtained with ADF <sup>S7</sup> and the default radii. The ZORA <sup>S9</sup> Hamiltonian was used. Values in red are reported from the main text for convenience. . . . .                                                                                          | S-8  |
| S6 | QTAIM bonding indicators obtained at the An–O (An = Pa, U) bond critical points and Bader charges, based on ADF <sup>S7</sup> calculations with the COSMO implicit solvation <sup>S6</sup> and the PBE0 exchange-correlation functional. <sup>S10</sup> Distances and delocalisation indices are reported from the main text for convenience. . . . . | S-9  |
| S7 | Mayer <sup>S11</sup> and Wiberg <sup>S12</sup> bond indices of the Pa–O and Pa–Cl bonds within the [PaO(Cl) <sub>5</sub> ] <sup>2-</sup> cluster, at the PBE+D3(BJ) solid-state geometry. Calculations were performed with ADF <sup>S7</sup> and the TZ2P basis sets. <sup>S13</sup> . . . . .                                                        | S-10 |
| S8 | Pa (5f and 6d orbitals) and O atomic orbital contributions to the $\sigma$ and $\pi$ Pa–O natural localized molecular orbitals (NLMOs) <sup>S14</sup> within [PaO(Cl) <sub>5</sub> ] <sup>2-</sup> cluster (same computational details as in Table S7). . . . .                                                                                       | S-10 |

|    |                                                                                                                                                                                                                                                                    |      |
|----|--------------------------------------------------------------------------------------------------------------------------------------------------------------------------------------------------------------------------------------------------------------------|------|
| S9 | Pa (5f and 6d orbitals) and Cl atomic orbital contributions to the $\sigma$ and $\pi$<br>Pa–Cl natural localized molecular orbitals (NLMOs) <sup>S14</sup> within $[\text{PaO}(\text{Cl})_5]^{2-}$<br>cluster (same computational details as in Table S7). . . . . | S-10 |
|----|--------------------------------------------------------------------------------------------------------------------------------------------------------------------------------------------------------------------------------------------------------------------|------|

Table S1: Integrated crystal orbital bond indices (ICOBIs)<sup>S1</sup> obtained at the optimized structures (see Tables 1 and 2). Mean values are reported when related bonds are crystallography independent.

|                                                       |      |                     |                     |
|-------------------------------------------------------|------|---------------------|---------------------|
| $[\text{C}_8\text{H}_{20}\text{N}]_2[\text{PaOCl}_5]$ | Pa–O | Pa–Cl <sub>ax</sub> | Pa–Cl <sub>eq</sub> |
| PBE+D3(BJ)                                            | 2.24 | 0.98                | 0.81                |

  

|                                                               |                   |  |      |
|---------------------------------------------------------------|-------------------|--|------|
| $(\text{C}_4\text{H}_{12}\text{N}_2)[\text{UO}_2\text{Cl}_4]$ | U–O <sub>yl</sub> |  | U–Cl |
| PBE+D3(BJ)                                                    | 2.17              |  | 0.85 |

  

|                                                                                                |                   |                  |      |
|------------------------------------------------------------------------------------------------|-------------------|------------------|------|
| $(\text{C}_4\text{H}_{12}\text{N}_2)_2[\text{UO}_2\text{Cl}_4(\text{H}_2\text{O})]\text{Cl}_2$ | U–O <sub>yl</sub> | U–O <sub>w</sub> | U–Cl |
| PBE+D3(BJ)                                                                                     | 2.32              | 0.36             | 0.63 |

For assessing the impact of the “environment”, bare  $[\text{PaO}]^{3+}$  and  $[\text{UO}_2]^{2+}$  systems have been optimized at the PBE level within large cubic boxes, ensuring more than 10 Å of distance between two molecular units. The resulting bond distances were 1.822 and 1.811 Å, respectively, together with ICOBIs of 2.97 and 2.66. These values serve as references to assess the impact of coordination in the crystal structures on the bonding of the  $[\text{PaO}]^{3+}$  and  $[\text{UO}_2]^{2+}$  subunits. This impact on bonding, referred to as  $\Delta\text{ICOB}$ I, was found to be  $-0.73$  for  $[\text{PaO}]^{3+}$  in  $[\text{C}_8\text{H}_{20}\text{N}]_2[\text{PaOCl}_5]$  and  $-0.49$  and  $-0.34$  in  $(\text{C}_4\text{H}_{12}\text{N}_2)[\text{UO}_2\text{Cl}_4]$  and  $(\text{C}_4\text{H}_{12}\text{N}_2)_2[\text{UO}_2\text{Cl}_4(\text{H}_2\text{O})]\text{Cl}_2$ , respectively.

Note that the ICObI is larger in  $(\text{C}_4\text{H}_{12}\text{N}_2)_2[\text{UO}_2\text{Cl}_4(\text{H}_2\text{O})]\text{Cl}_2$  than in  $(\text{C}_4\text{H}_{12}\text{N}_2)[\text{UO}_2\text{Cl}_4]$  by 0.15, corroborating the water-induced effective bond reinforcement observed by Rajapaksha et al.<sup>S15</sup>. This bond reinforcement is concomitant with a reduction of the U–Cl ICObI, meaning that it is in fact indirect: by weakening the in-plane bonds with water addition, the uranyl bonds are effectively less destabilized, thus appearing reinforced.

Note that the valence 7p levels of Pa and U are omitted from the ICObI analysis by absence of such basis functions in the used program<sup>S16</sup> (the procedure requires projection of the plane waves onto a localized basis). Since these atomic levels only have a limited impact on bonding, their omission does not significantly affect our analysis.

Table S2: Benchmark of ten exchange-correlation (XC) functionals based on the Abinit code<sup>S2</sup> for selected protactinium molecular systems. Only the Pa–O bond distance (Å) is reported.

| XC functional               | [PaO] <sup>3+</sup> | PaOF <sub>3</sub> (H <sub>2</sub> O) <sub>3</sub> | [PaO(C <sub>2</sub> O <sub>4</sub> ) <sub>3</sub> ] <sup>3-</sup> |
|-----------------------------|---------------------|---------------------------------------------------|-------------------------------------------------------------------|
| PW91 <sup>S17</sup>         | 1.710               | 1.817                                             | 1.851                                                             |
| LDA (Wigner) <sup>S18</sup> | 1.723               | 1.832                                             | 1.867                                                             |
| PBE <sup>S19</sup>          | 1.722               | 1.833                                             | 1.869                                                             |
| HTCH93 <sup>S20</sup>       | 1.710               | 1.813                                             | 1.842                                                             |
| HTCH120 <sup>S21</sup>      | 1.710               | 1.814                                             | 1.847                                                             |
| HTCH147 <sup>S21</sup>      | 1.710               | 1.813                                             | 1.845                                                             |
| HTCH407 <sup>S22</sup>      | 1.708               | 1.811                                             | 1.848                                                             |
| GGA (Wu) <sup>S23</sup>     | 1.715               | 1.824                                             | 1.860                                                             |
| HTBS <sup>S24</sup>         | 1.743               | 1.865                                             | 1.887                                                             |
| MOHLYP <sup>S25</sup>       | 1.730               | 1.842                                             | 1.874                                                             |

Table S3: Role of implicit solvation (C-PCM<sup>S3</sup>) on the Pa–O bond distance (Å) obtained with Gaussian<sup>S4</sup> and the default radii (UFF<sup>S5</sup>).

| $[\text{PaO}]^{3+}$            | Gas phase | C-PCM |
|--------------------------------|-----------|-------|
| B3PW91 <sup>S26</sup>          | 1.689     | 1.759 |
| B3LYP <sup>S27</sup>           | 1.697     | 1.771 |
| PBE <sup>S19</sup>             | 1.717     | 1.782 |
| PBE0 <sup>S10</sup>            | 1.681     | 1.752 |
| PBE0+D3(BJ) <sup>S10,S28</sup> | 1.681     | 1.752 |
| MP2 <sup>S29</sup>             | 1.714     | 1.766 |

| $[\text{PaO}(\text{C}_2\text{O}_4)_3]^{3-}$ | Gas phase | C-PCM |
|---------------------------------------------|-----------|-------|
| B3PW91 <sup>S26</sup>                       | 1.850     | 1.856 |
| B3LYP <sup>S27</sup>                        | 1.862     | 1.867 |
| PBE <sup>S19</sup>                          | 1.874     | 1.881 |
| PBE0 <sup>S10</sup>                         | 1.843     | 1.849 |
| PBE0+D3(BJ) <sup>S10,S28</sup>              | 1.844     | 1.849 |
| MP2 <sup>S29</sup>                          | 1.857     | 1.857 |

The def2-TZVP basis sets<sup>S30</sup> were used on all atoms except for Pa, which was treated with the ECP60MWB energy-consistent pseudopotential<sup>S31</sup> along with its corresponding segmented basis set.<sup>S32</sup> Overall, a bond lengthening of  $\sim 0.07$  Å is observed for  $[\text{PaO}]^{3+}$  and  $\sim 0.006$  Å for  $[\text{PaO}(\text{C}_2\text{O}_4)_3]^{3-}$ , respectively. Notably, there was minimal variation when changing the underlying electronic structure theory method.

Additionally, calculations were conducted in the gas phase using Molpro,<sup>S33</sup> yielding a scalar-relativistic CCSD(T)<sup>S34</sup> value of 1.703 Å for  $[\text{PaO}]^{3+}$ . The MP2 and B3LYP calculations were also repeated for cross-checking, leading with this setup to 1.714 and 1.698 Å, respectively; values which are identical to those obtained using the Gaussian software.

Table S4: Role of implicit solvation (COSMO<sup>S6</sup>) on the Pa–O bond distance (Å) obtained with ADF<sup>S7</sup> and the default radii.<sup>S8</sup> The ZORA<sup>S9</sup> Hamiltonian was used. Values in red are reported from the main text for convenience.

| $[\text{PaO}]^{3+}$  | Relativity | Gas phase | COSMO |
|----------------------|------------|-----------|-------|
| B3LYP <sup>S27</sup> | Scalar     | 1.705     | 1.729 |
|                      | Spin-orbit | 1.707     | 1.731 |
| PBE0 <sup>S10</sup>  | Scalar     | 1.688     | 1.710 |
|                      | Spin-orbit | 1.690     | 1.713 |

  

| $[\text{PaO}(\text{C}_2\text{O}_4)_3]^{3-}$ | Relativity | Gas phase | COSMO |
|---------------------------------------------|------------|-----------|-------|
| B3LYP <sup>S27</sup>                        | Scalar     | 1.871     | 1.878 |
|                                             | Spin-orbit | 1.873     | 1.881 |
| PBE0 <sup>S10</sup>                         | Scalar     | 1.852     | 1.858 |
|                                             | Spin-orbit | 1.854     | 1.862 |

The TZ2P basis sets<sup>S13</sup> were used on all atoms. By comparing Table S3 and Table S4, it is clear that the COSMO model leads to a lesser impact of solvation on the Pa–O bond distance than the C-PCM one. Test calculations have shown that this is essentially due to the use of the default UFF radii (rescaled by the 1.1 default  $\alpha$  value). Despite this moderate discrepancy, the previous trend holds (solvation-induced bond lengthening).

Table S5: Role of implicit solvation (COSMO<sup>S6</sup>) on the U–O bond distance(s) (Å) obtained with ADF<sup>S7</sup> and the default radii. The ZORA<sup>S9</sup> Hamiltonian was used. Values in red are reported from the main text for convenience.

| $[\text{UO}_2]^{2+}$                         | Relativity | Gas phase | COSMO             |
|----------------------------------------------|------------|-----------|-------------------|
| PBE0 <sup>S10</sup>                          | Scalar     | 1.684     | <b>1.702</b>      |
|                                              | Spin-orbit | 1.687     | 1.705             |
| $[\text{UO}_2\text{Cl}_4]^{2-}$              | Relativity | Gas phase | COSMO             |
| PBE0 <sup>S10</sup>                          | Scalar     | 1.763     | <b>1.766</b>      |
|                                              | Spin-orbit | 1.767     | 1.771             |
| $[\text{UO}_2(\text{C}_2\text{O}_4)_3]^{4-}$ | Relativity | Gas phase | COSMO             |
| PBE0 <sup>S10</sup>                          | Scalar     | 1.779(3)  | <b>1.7815(15)</b> |
|                                              | Spin-orbit | 1.783(3)  | 1.786(2)          |

The TZ2P basis sets<sup>S13</sup> were used on all atoms. As other deviation values reported in parenthesis in the main text for mean distances, the standard deviations have been computed using the following formula:

$$\sigma = \sqrt{\frac{1}{N} \sum_{i=1}^N (d_i - \bar{d})^2} \quad (1)$$

where  $N$  is the number of distances entering the calculation of the mean  $\bar{d}$  value. In other words, no Bessel’s correction was applied.

Table S6: QTAIM bonding indicators obtained at the An–O (An = Pa, U) bond critical points and Bader charges, based on ADF<sup>S7</sup> calculations with the COSMO implicit solvation<sup>S6</sup> and the PBE0 exchange-correlation functional.<sup>S10</sup> Distances and delocalisation indices are reported from the main text for convenience.

| System                                       | $d$ (Å)    | $\rho$ , a.u. | $\nabla^2\rho$ | G, a.u. | V, a.u. | $ V /G$ | H, a.u. | $q(\text{An})$ , a.u. | $q(\text{X})$ , a.u. | $\delta$ |
|----------------------------------------------|------------|---------------|----------------|---------|---------|---------|---------|-----------------------|----------------------|----------|
| $[\text{PaO}]^{3+}$                          | 1.710      | 0.36          | 0.33           | 0.58    | −1.07   | 1.84    | −0.50   | 3.69                  | −0.69                | 2.33     |
| $[\text{PaO}(\text{C}_2\text{O}_4)_3]^{3-}$  | 1.858      | 0.25          | 0.36           | 0.34    | −0.59   | 1.74    | −0.25   | 3.09                  | −1.14                | 1.69     |
| $[\text{UO}_2]^{2+}$                         | 1.702      | 0.36          | 0.39           | 0.59    | −1.10   | 1.86    | −0.49   | 3.53                  | −0.77                | 2.15     |
| $[\text{UO}_2\text{Cl}_4]^{2-}$              | 1.766      | 0.30          | 0.36           | 0.46    | −0.83   | 1.80    | −0.37   | 2.93                  | −0.97                | 1.89     |
| $[\text{UO}_2(\text{C}_2\text{O}_4)_3]^{4-}$ | 1.7815(15) | 0.29          | 0.36           | 0.44    | −0.79   | 1.80    | −0.35   | 2.41                  | −0.73                | 1.84     |

Table S7: Mayer<sup>S11</sup> and Wiberg<sup>S12</sup> bond indices of the Pa–O and Pa–Cl bonds within the  $[\text{PaO}(\text{Cl})_5]^{2-}$  cluster, at the PBE+D3(BJ) solid-state geometry. Calculations were performed with ADF<sup>S7</sup> and the TZ2P basis sets.<sup>S13</sup>

|        | Pa–O | Pa–Cl <sub>ax</sub> | Pa–Cl <sub>eq</sub> |
|--------|------|---------------------|---------------------|
| Mayer  | 2.02 | 0.91                | 0.79                |
| Wiberg | 2.07 | 1.03                | 0.91                |

Table S8: Pa (5f and 6d orbitals) and O atomic orbital contributions to the  $\sigma$  and  $\pi$  Pa–O natural localized molecular orbitals (NLMOs)<sup>S14</sup> within  $[\text{PaO}(\text{Cl})_5]^{2-}$  cluster (same computational details as in Table S7).

| $\sigma$ |        |        | $\pi$  |        |        |
|----------|--------|--------|--------|--------|--------|
| Pa(5f)   | Pa(6d) | O(s/p) | Pa(5f) | Pa(6d) | O(s/p) |
| 16.2     | 6.4    | 76.4   | 10.7   | 9.3    | 79.7   |

Table S9: Pa (5f and 6d orbitals) and Cl atomic orbital contributions to the  $\sigma$  and  $\pi$  Pa–Cl natural localized molecular orbitals (NLMOs)<sup>S14</sup> within  $[\text{PaO}(\text{Cl})_5]^{2-}$  cluster (same computational details as in Table S7).

|                  | $\sigma$ |        |         | $\pi$  |        |         |
|------------------|----------|--------|---------|--------|--------|---------|
|                  | Pa(5f)   | Pa(6d) | Cl(s/p) | Pa(5f) | Pa(6d) | Cl(s/p) |
| Cl <sub>ax</sub> | 8.1      | 6.2    | 83.5    | 3.7    | 3.9    | 92.2    |
| Cl <sub>eq</sub> | 4.7      | 7.2    | 85.3    |        |        |         |

To cross-check our previous analysis of the solid-state  $[\text{C}_8\text{H}_{20}\text{N}]_2[\text{PaOCl}_5]$  compound based on ICOBIs (see Table S1 and the related discussion), we have also performed bonding analyses within the molecular quantum chemistry framework, based on the  $[\text{PaO}(\text{Cl})_5]^{2-}$  cluster, defined at the solid-state geometry. Clearly, the deviation to the ideal triple bond is confirmed with both the Mayer<sup>S11</sup> and Wiberg<sup>S12</sup> bond indices and the specificity of the Pa–Cl<sub>ax</sub> bond is also reproduced. We have also computed atomic contributions per shell to the  $\sigma$  and  $\pi$  bonds between the atoms of interest, when applicable (see Tables S8 and S9). While both the Pa–O and Pa–Cl<sub>ax</sub> bonds display actual  $\pi$  character, it is absent from the Pa–Cl<sub>eq</sub> bonds. This, together with the shorter Pa–Cl<sub>eq</sub> bond distance (compared to the Pa–Cl<sub>ax</sub> ones), is in fact a signature for the inverse *trans* effect, expected for  $[\text{C}_8\text{H}_{20}\text{N}]_2[\text{PaOCl}_5]$ .<sup>S35</sup>

## References

- (S1) Müller, P. C.; Ertural, C.; Hempelmann, J.; Dronskowski, R. Crystal Orbital Bond Index: Covalent Bond Orders in Solids. *J. Phys. Chem. C* **2021**, *125*, 7959–7970, DOI: 10.1021/acs.jpcc.1c00718.
- (S2) Gonze, X.; Amadon, B.; Antonius, G.; Arnardi, F.; Baguet, L.; Beuken, J.-M.; Bieder, J.; Bottin, F.; Bouchet, J.; Bousquet, E.; Brouwer, N.; Bruneval, F.; Brunin, G.; Cavignac, T.; Charraud, J.-B.; Chen, W.; Côté, M.; Cottenier, S.; Denier, J.; Geneste, G.; Ghosez, P.; Giantomassi, M.; Gillet, Y.; Gingras, O.; Hamann, D. R.; Hautier, G.; He, X.; Helbig, N.; Holzwarth, N.; Jia, Y.; Jollet, F.; Lafargue-Dit-Hauret, W.; Lejaeghere, K.; Marques, M. A.; Martin, A.; Martins, C.; Miranda, H. P.; Naccarato, F.; Persson, K.; Petretto, G.; Planes, V.; Pouillon, Y.; Prokhorenko, S.; Ricci, F.; Rignanese, G.-M.; Romero, A. H.; Schmitt, M. M.; Torrent, M.; van Setten, M. J.; Van Troeye, B.; Verstraete, M. J.; Zérah, G.; Zwanziger, J. W. The Abinit project: Impact, environment and recent developments. *Comput. Phys. Commun.* **2020**, *248*, 107042, DOI: 10.1016/j.cpc.2019.107042.
- (S3) Cossi, M.; Rega, N.; Scalmani, G.; Barone, V. Energies, structures, and electronic properties of molecules in solution with the C-PCM solvation model. *J. Comput. Chem.* **2003**, *24*, 669–681, DOI: 10.1002/jcc.10189.
- (S4) Frisch, M. J.; Trucks, G. W.; Schlegel, H. B.; Scuseria, G. E.; Robb, M. A.; Cheeseman, J. R.; Scalmani, G.; Barone, V.; Petersson, G. A.; Nakatsuji, H.; Li, X.; Caricato, M.; Marenich, A. V.; Bloino, J.; Janesko, B. G.; Gomperts, R.; Menucci, B.; Hratchian, H. P.; Ortiz, J. V.; Izmaylov, A. F.; Sonnenberg, J. L.; Williams-Young, D.; Ding, F.; Lipparini, F.; Egidi, F.; Goings, J.; Peng, B.; Petrone, A.; Henderson, T.; Ranasinghe, D.; Zakrzewski, V. G.; Gao, J.; Rega, N.; Zheng, G.; Liang, W.; Hada, M.; Ehara, M.; Toyota, K.; Fukuda, R.; Hasegawa, J.; Ishida, M.; Nakajima, T.; Honda, Y.; Kitao, O.; Nakai, H.; Vreven, T.; Throssell, K.; Mont-

- gomery, J. A., Jr.; Peralta, J. E.; Ogliaro, F.; Bearpark, M. J.; Heyd, J. J.; Brothers, E. N.; Kudin, K. N.; Staroverov, V. N.; Keith, T. A.; Kobayashi, R.; Normand, J.; Raghavachari, K.; Rendell, A. P.; Burant, J. C.; Iyengar, S. S.; Tomasi, J.; Cossi, M.; Millam, J. M.; Klene, M.; Adamo, C.; Cammi, R.; Ochterski, J. W.; Martin, R. L.; Morokuma, K.; Farkas, O.; Foresman, J. B.; Fox, D. J. Gaussian~16 Revision C.01. 2016; Gaussian Inc. Wallingford CT.
- (S5) Rappe, A. K.; Casewit, C. J.; Colwell, K. S.; Goddard, W. A. I.; Skiff, W. M. UFF, a full periodic table force field for molecular mechanics and molecular dynamics simulations. *J. Am. Chem. Soc.* **1992**, *114*, 10024–10035, DOI: 10.1021/ja00051a040.
- (S6) Pye, C. C.; Ziegler, T. An Implementation of the Conductor-like Screening Model of Solvation within the Amsterdam Density Functional Package. *Theor. Chem. Acc.* **1999**, *101*, 396–408, DOI: 10.1007/s002140050457.
- (S7) te Velde, G.; Bickelhaupt, F. M.; Baerends, E. J.; Fonseca Guerra, C.; van Gisbergen, S. J. A.; Snijders, J. G.; Ziegler, T. Chemistry with ADF. *J. Comput. Chem.* **2001**, *22*, 931–967, DOI: 10.1002/jcc.1056.
- (S8) Allinger, N. L.; Zhou, X.; Bergsma, J. Molecular mechanics parameters. *J. Mol. Struct. THEOCHEM* **1994**, *312*, 69–83, DOI: 10.1016/S0166-1280(09)80008-0.
- (S9) van Lenthe, E.; Snijders, J. G.; Baerends, E. J. The zero-order regular approximation for relativistic effects: The effect of spin–orbit coupling in closed shell molecules. *J. Chem. Phys.* **1996**, *105*, 6505–6516, DOI: 10.1063/1.472460.
- (S10) Adamo, C.; Scuseria, G. E.; Barone, V. Accurate excitation energies from time-dependent density functional theory: Assessing the PBE0 model. *J. Chem. Phys.* **1999**, *111*, 2889–2899, DOI: 10.1063/1.479571.
- (S11) Mayer, I. Bond order and valence indices: A personal account. *J. Comput. Chem.* **2007**, *28*, 204–221, DOI: <https://doi.org/10.1002/jcc.20494>.

- (S12) Wiberg, K. B. Application of the popple-santry-segal CNDO method to the cyclopropylcarbiny and cyclobutyl cation and to bicyclobutane. *Tetrahedron* **1968**, *24*, 1083–1096.
- (S13) Van Lenthe, E.; Baerends, E. J. Optimized Slater-type basis sets for the elements 1–118. *J. Comput. Chem.* **2003**, *24*, 1142–1156, DOI: 10.1002/jcc.10255.
- (S14) Reed, A. E.; Weinhold, F. Natural localized molecular orbitals. *J. Chem. Phys.* **1985**, *83*, 1736–1740, DOI: 10.1063/1.449360.
- (S15) Rajapaksha, H.; Mason, S. E.; Forbes, T. Z. Synthesis, Characterization, and Density Functional Theory Investigation of the Solid-State  $[\text{UO}_2\text{Cl}_4(\text{H}_2\text{O})]^{2-}$  Complex. *Inorg. Chem.* **2023**, *62*, 14318–14325, DOI: 10.1021/acs.inorgchem.3c01725.
- (S16) Maintz, S.; Deringer, V. L.; Tchougréeff, A. L.; Dronskowski, R. LOBSTER: A tool to extract chemical bonding from plane-wave based DFT. *J. Comput. Chem.* **2016**, *37*, 1030–1035, DOI: <https://doi.org/10.1002/jcc.24300>.
- (S17) Perdew, J. P.; Chevary, J. A.; Vosko, S. H.; Jackson, K. A.; Pederson, M. R.; Singh, D. J.; Fiolhais, C. Atoms, molecules, solids, and surfaces: Applications of the generalized gradient approximation for exchange and correlation. *Phys. Rev. B* **1992**, *46*, 6671–6687, DOI: 10.1103/PhysRevB.46.6671.
- (S18) Wigner, E. Effects of the electron interaction on the energy levels of electrons in metals. *Trans. Faraday Soc.* **1938**, *34*, 678–685, DOI: 10.1039/TF9383400678.
- (S19) Perdew, J. P.; Burke, K.; Ernzerhof, M. Generalized Gradient Approximation Made Simple. *Phys. Rev. Lett.* **1997**, *78*, 1396–1396, DOI: 10.1103/PhysRevLett.78.1396.
- (S20) Hamprecht, F. A.; Cohen, A. J.; Tozer, D. J.; Handy, N. C. Development and assessment of new exchange-correlation functionals. *J. Chem. Phys.* **1998**, *109*, 6264–6271, DOI: 10.1063/1.477267.

- (S21) Boese, A. D.; Doltsinis, N. L.; Handy, N. C.; Sprik, M. New generalized gradient approximation functionals. *J. Chem. Phys.* **2000**, *112*, 1670–1678, DOI: 10.1063/1.480732.
- (S22) Boese, A. D.; Handy, N. C. A new parametrization of exchange–correlation generalized gradient approximation functionals. *J. Chem. Phys.* **2001**, *114*, 5497–5503, DOI: 10.1063/1.1347371.
- (S23) Wu, Z.; Cohen, R. E. More accurate generalized gradient approximation for solids. *Phys. Rev. B* **2006**, *73*, 235116, DOI: 10.1103/PhysRevB.73.235116.
- (S24) Haas, P.; Tran, F.; Blaha, P.; Schwarz, K. Construction of an optimal GGA functional for molecules and solids. *Phys. Rev. B* **2011**, *83*, 205117, DOI: 10.1103/PhysRevB.83.205117.
- (S25) Schultz, N. E.; Zhao, Y.; Truhlar, D. G. Density Functionals for Inorganometallic and Organometallic Chemistry. *J. Phys. Chem. A* **2005**, *109*, 11127–11143, DOI: 10.1021/jp0539223.
- (S26) Becke, A. D. Density-functional thermochemistry. III. The role of exact exchange. *J. Chem. Phys.* **1993**, *98*, 5648–5652, DOI: 10.1063/1.464913.
- (S27) Stephens, P. J.; Devlin, F. J.; Chabalowski, C. F.; Frisch, M. J. Ab Initio Calculation of Vibrational Absorption and Circular Dichroism Spectra Using Density Functional Force Fields. *J. Chem. Phys.* **1994**, *98*, 11623–11627, DOI: 10.1021/j100096a001.
- (S28) Grimme, S.; Ehrlich, S.; Goerigk, L. Effect of the damping function in dispersion corrected density functional theory. *J. Comput. Chem.* **2011**, *32*, 1456–1465, DOI: 10.1002/jcc.21759.
- (S29) Møller, C.; Plesset, M. S. Note on an Approximation Treatment for Many-Electron Systems. *Phys. Rev.* **1934**, *46*, 618–622, DOI: 10.1103/PhysRev.46.618.

- (S30) Weigend, F.; Ahlrichs, R. Balanced basis sets of split valence, triple zeta valence and quadruple zeta valence quality for H to Rn: Design and assessment of accuracy. *Phys. Chem. Chem. Phys.* **2005**, *7*, 3297–3305, DOI: 10.1039/B508541A.
- (S31) Küchle, W.; Dolg, M.; Stoll, H.; Preuss, H. Energy-adjusted pseudopotentials for the actinides. Parameter sets and test calculations for thorium and thorium monoxide. *J. Chem. Phys.* **1994**, *100*, 7535–7542, DOI: 10.1063/1.466847.
- (S32) Cao, X.; Dolg, M.; Stoll, H. Valence basis sets for relativistic energy-consistent small-core actinide pseudopotentials. *J. Chem. Phys.* **2003**, *118*, 487–496, DOI: 10.1063/1.1521431.
- (S33) Werner, H.-J.; Knowles, P. J.; Knizia, G.; Manby, F. R.; Schütz, M.; Celani, P.; Györffy, W.; Kats, D.; Korona, T.; Lindh, R.; Mitrushenkov, A.; Rauhut, G.; Shamasundar, K. R.; Adler, T. B.; Amos, R. D.; Bennie, S. J.; Bernhardsson, A.; Berning, A.; Cooper, D. L.; Deegan, M. J. O.; Dobbyn, A. J.; Eckert, F.; Goll, E.; Hampel, C.; Hesselmann, A.; Hetzer, G.; Hrenar, T.; Jansen, G.; Köppl, C.; Lee, S. J. R.; Liu, Y.; Lloyd, A. W.; Ma, Q.; Mata, R. A.; May, A. J.; McNicholas, S. J.; Meyer, W.; Miller III, T. F.; Mura, M. E.; Nicklass, A.; O’Neill, D. P.; Palmieri, P.; Peng, D.; Pflüger, K.; Pitzer, R.; Reiher, M.; Shiozaki, T.; Stoll, H.; Stone, A. J.; Tarroni, R.; Thorsteinsson, T.; Wang, M.; Welborn, M. MOLPRO, a package of ab initio programs, version 2023.2.
- (S34) Purvis, I., George D.; Bartlett, R. J. A full coupled-cluster singles and doubles model: The inclusion of disconnected triples. *J. Chem. Phys.* **1982**, *76*, 1910–1918, DOI: 10.1063/1.443164.
- (S35) Fryer-Kanssen, I.; Kerridge, A. Elucidation of the Inverse Trans Influence in Uranyl and Its Imido and Carbene Analogues via Quantum Chemical Simulation. *Chem. Commun.* **2018**, *54*, 9761–9764, DOI: 10.1039/C8CC06088F.
